# Supplementary material for: Short-Term Synaptic Plasticity Stabilizes Goal-Conditioned Dynamics in a Prefrontal Cortex-Inspired Reservoir Model for Multistep Goal-Directed Action Planning
Source: arXiv:2606.03481 source file (2026-11-29)
Supplement: Supplementary file 1 [file preamble_supplement.tex]

\makeatletter\newcommand{\ComposeFinalParagraphSpace}{\bigskip}
\ifdefined\FinalTabularBox\else\newbox\FinalTabularBox\fi
\newcommand{\ComposeAppendixSetup}{%
  \renewcommand{\thefigure}{S\arabic{figure}}%
  \renewcommand{\theHfigure}{S\arabic{figure}}\setcounter{figure}{0}%
  \renewcommand{\thetable}{S\arabic{table}}%
  \renewcommand{\theHtable}{S\arabic{table}}\setcounter{table}{0}%
  \setcounter{topnumber}{4}\setcounter{bottomnumber}{3}\setcounter{totalnumber}{6}%
  \setlength{\textfloatsep}{19pt plus 2pt minus 4pt}\setlength{\@fpsep}{20pt}}
\newenvironment{composegraphic}{\hbox\bgroup}{\egroup}
\newcommand{\ComposeCaption}[1]{%
  \vskip3pt\setbox0=\vbox{\hsize=\linewidth\@parboxrestore\linewidth=\hsize
    \def\baselinestretch{1}\fontsize{9}{11}\selectfont\normalbaselines
    \parindent=0pt\parskip=0pt\noindent#1\par}%
  \nointerlineskip\hbox{\box0}}
\newenvironment{composetable}{%
  \setbox0=\vbox\bgroup\textwidth=\linewidth\hsize=\textwidth
    \@parboxrestore\linewidth=\hsize\normalsize\normalbaselines
    \parindent=0pt\parskip=0pt\hfuzz=0pt\noindent
}{%
  \par\egroup%
  \nointerlineskip\box0}
\newenvironment{composelabel}{%
  \setbox0=\hbox\bgroup\def\baselinestretch{1}%
    \fontsize{9}{11}\selectfont\strut%
}{%
  \egroup\ifdim\wd0>\linewidth\fi
  \ifdim\dimexpr\ht0+\dp0\relax>11.0001pt
    \fi
  \vbox to11pt{\offinterlineskip\box0\vss}}
\newcommand{\ComposeNumberHeader}[1]{%
  \refstepcounter{figure}%
  \begin{composelabel}\textbf{Figure~\thefigure:#1}\end{composelabel}}
\newenvironment{composerow}{\hbox\bgroup}{\egroup}
\newenvironment{composecell}[1][121.254]{%
  \vtop\bgroup\hsize=#1mm\linewidth=\hsize
    \parindent=0pt\parskip=0pt\offinterlineskip\hbox{}
}{\egroup}
\def\ComposePageMeta#1|#2|#3\relax{\def\ComposePageKey{#1}\def\ComposePageIndex{#2}\def\ComposePageAnchor{#3}}
\newenvironment{composepage}[1][]{%
  \ComposePageMeta#1\relax
  \ifnum\ComposePageIndex>1
    \renewcommand{\theHfigure}{\arabic{figure}.\ComposePageAnchor}\addtocounter{figure}{-1}\fi
  \def\@makecaption##1##2{\offinterlineskip\ComposeCaption{##1: ##2}}%
  \setbox2=\vbox\bgroup\hsize=121.254mm\linewidth=\hsize
    \parindent=0pt\parskip=0pt\offinterlineskip
}{%
  \egroup%
  \ifdim\dimexpr\ht2+\dp2\relax>\textheight
    \centering\box2%
  \else\centering\box2\fi}
\newcommand{\ComposePart}[1]{\def\fnum@figure{\figurename\nobreakspace\thefigure#1}}\newcommand{\ComposeKeep}[1]{#1}\newcommand{\ComposePartLabel}[1]{\begingroup\protected@edef\@currentlabel{\thefigure#1}\label{\ComposePageKey:part#1}\endgroup}\makeatother
